# Supplementary material for: Nonreciprocal Dzyaloshinskii-Moriya magnetoacoustic waves
Source: arXiv:2004.03535 ancillary file (2020-12-02)
Supplement: Supplementary file 1 [file Supplemental_Material.pdf]

# SUPPLEMENTAL MATERIAL

# Nonreciprocal Dzyaloshinskii–Moriya Magnetoacoustic Waves

M. Küß,* A. Hörner, and A. Wixforth

*Experimental Physics I, Institute of Physics,*
*University of Augsburg, 86135 Augsburg, Germany*

M. Heigl and M. Albrecht

*Experimental Physics IV, Institute of Physics,*
*University of Augsburg, 86135 Augsburg, Germany*

L. Flacke and M. Weiler†

*Walther-Meißner-Institut, Bayerische Akademie*
*der Wissenschaften, 85748 Garching, Germany and*
*Physics-Department, Technical University Munich, 85748 Garching, Germany*

## [S.1] SAMPLE PREPARATION

The interdigital transducers (IDTs) in Fig. S1 were fabricated on a piezoelectric Y-cut Z-propagation $LiNbO_3$ substrate with electron beam lithography and electron beam evaporation of 5 nm Ti and 70 nm of Al. The $LiNbO_3$ substrate supports Rayleigh type SAWs [1]. To attain high SAW transmission at high frequencies and wide transmission bands ($\propto 1/n$), the aperture of the IDT is 200 $\mu$m and the number of finger pairs is $n = 3$. In a second lithography step, rectangular-shaped $Co_{40}Fe_{40}B_{20}(d)/Pt(3)/Si_3N_4(3)$ films with 1.4 nm $\leq d \leq$ 5.0 nm and a $Co_{40}Fe_{40}B_{20}(2)/Si_3N_4(3)$ film (numbers are the nominal thickness in nm) were deposited at room temperature by magnetron sputtering (base pressure $< 10^{-7}$ mbar) between the IDTs. The Ar pressure was kept constant at $5 \times 10^{-3}$ mbar during the deposition process and the sample holder was rotating during sputtering. The individual layer thicknesses were determined using a calibrated deposition rate.

## [S.2] THEORETICAL MODEL

In this section, we derive the theoretical model being used to fit the SAW transmission $\Delta S_{ij}$, with $ij \in \{21, 12\}$ and to extract the considered properties of the studied thin films. We employ the same Cartesian coordinate system as in the main text, with the x-axis being

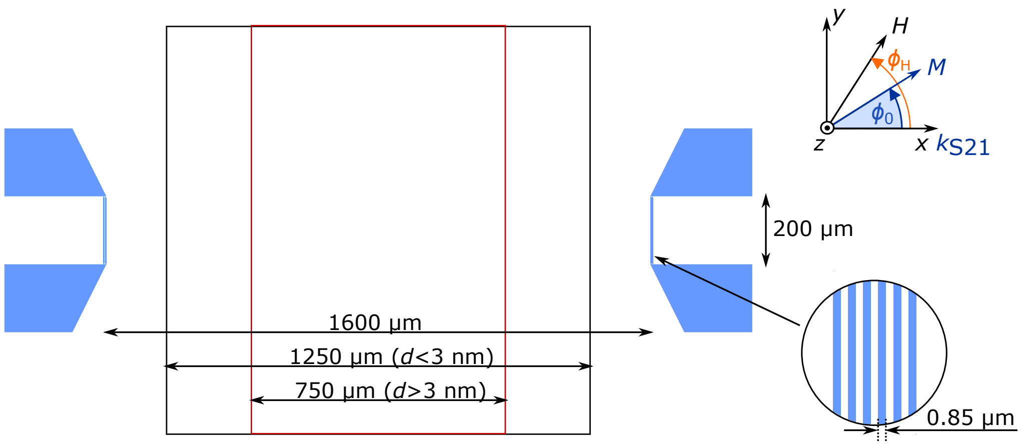


FIG. S1. Drawing to scale of the lithography pattern. The length of the magnetic films $l_f$ is reduced for the thicker films $d = 3.5$ nm, 5 nm to avoid very high attenuation of the SAW due to SAW-SW interaction and to optimize the signal-to-noise ratio.

parallel to the SAW propagation direction $k_{\mathrm{S21}}$, the z-axis is normal to the magnetic film plane and the y-axis lies in the magnetic film plane.

### Magnetoacoustic driving fields

Following the approach by Dreher et al. [2] the in-plane $h_{\mathrm{ip}}$ and out-of-plane $h_{\mathrm{oop}}$ magnetoelastic driving field components of a Rayleigh wave in a magnetic film with in-plane aligned magnetization are given by

$$\mathbf{h}(x,z,t) = \begin{pmatrix} h_{\mathrm{oop}}(x,z,t) \\ h_{\mathrm{ip}}(x,z,t) \end{pmatrix} = \frac{1}{\mu_0} \begin{pmatrix} 2b_2\epsilon_{xz}(x,z,t)\cos\phi_0 \\ 2b_1\epsilon_{xx}(x,z,t)\cos\phi_0\sin\phi_0 \end{pmatrix}. \tag{1}$$

Here, $b_1$ and $b_2$ are the magnetoelastic coupling constants, $\epsilon_{ij}(x,z,t) = \epsilon_{ij,0}(x,z)\mathrm{e}^{i(kx-\omega t)}$ are the longitudinal ($ij = xx$) and vertical shear ($ij = xz$) strain components of the SAW with the complex amplitudes $\epsilon_{ij,0}(x,z)$ the angular frequency $\omega$, the wave vector $k$ and $\phi_0$ denotes the orientation of the equilibrium in-plane magnetization direction with respect to the x-axis.

First, we carry out an established finite element eigenfrequency study with Comsol [3] at $\sim 6.9$ GHz and the parameters in Table SI to investigate the magnitude and phase behavior of $\epsilon_{xx}$ and $\epsilon_{xz}$ in more detail. The strain as a function of x-position at an arbitrary point in time $t^*$ at the top surface $\epsilon_{ij}(x, z = 0, t = t^*)$ and the magnitude of the strain in the z-direction, $|\epsilon_{ij,0}(x = 0, z)|$ are depicted for the two limiting cases of a pure $LiNbO_3$ substrate in Figs. S2(a, d) and for a pure $LiNbO_3$ substrate with a perfectly conducting overlayer of zero thickness in Figs. S2(b, e). Panels (c, f) show the results for the $LiNbO_3$/CoFeB(2)/$Si_3N_4$(3) sample for the magnetic film center plane $\epsilon_{ij}(x, z = -4\ \mathrm{nm}, t = t^*)$ and $|\epsilon_{ij,0}(x = 0, z)|$. Here, we assumed an ideal conductive CoFeB film, which is justified by the experimentally determined SAW propagation velocity of $c = (3394 \pm 15)$ m/s, corresponding to the velocity of a metalized $LiNbO_3$ substrate of $c_{\mathrm{sc}} = 3404$ m/s [1]. With the material parameters in Table SI, the phase of the strain $\epsilon_{xz}$ is shifted by $+90°$ with respect to $\epsilon_{xx}$ and the magnitude of $\epsilon_{xz}$ is $(8 \pm 6)\%$ of $\epsilon_{xx}$. Note, that this ratio depends critically on the material properties of the ultrathin sputtered films, resulting in the rather large error of 6%. Because of the ultrathin films discussed in this report ($d \leq 5$ nm), we neglect the z-dependence of strain and lattice displacement in the magnetic films in the following discussion.

TABLE SI. The assumed thin film parameters, that were used in the finite element method simulation. The parameters for the anisotropic single-crystal $LiNbO_3$ are taken from Ref. [4].

| | $Co_{40}Fe_{40}B_{20}$ [5, 6] | $Si_3N_4$ [4] | Pt [4] |
|---|---|---|---|
| Density (kg/m$^3$) | 7156 | 3100 | 21450 |
| Young's modulus ($10^9$ N/m) | 160 | 250 | 168 |
| Poisson's ratio | 0.3 | 0.23 | 0.38 |

Since the constants $\tilde{a}_{xx} = \frac{\epsilon_{xx,0}}{|u_{z,0}||k|}$, $\tilde{a}_{xz} = \frac{\epsilon_{xz,0}}{|u_{z,0}||k|}$ can be determined with the finite element method, where $u_{z,0}$ is the amplitude of the lattice displacement in the z-direction, we substitute

$$\begin{aligned}\epsilon_{xx}(x,t) &= \epsilon_{xx,0}(x)\mathrm{e}^{i(kx-\omega t)} = \tilde{a}_{xx}|k||u_{z,0}(x)|\mathrm{e}^{i(kx-\omega t)}\\ \epsilon_{xz}(x,t) &= \epsilon_{xz,0}(x)\mathrm{e}^{i(kx-\omega t)} = \tilde{a}_{xz}|k||u_{z,0}(x)|\mathrm{e}^{i(kx-\omega t)}.\end{aligned} \tag{2}$$

From the simulation, we obtain for the pure $LiNbO_3$ substrate in Figs. S2(a, d) $\tilde{a}_{xx} = 0.68$, which is in agreement with literature $|\tilde{a}_{xx}| = \frac{1}{|u_{z,0}||k|}\left|\frac{\partial}{\partial x}u_{x,0}\mathrm{e}^{i(kx-\omega t)}\right| = \frac{|u_{x,0}|}{|u_{z,0}|} = \frac{2}{3}$ [7], where $u_{x,0}$ is the amplitude of lattice displacement in the x-direction. Additionally, the obtained values $\tilde{a}_{xx}$ and $\tilde{a}_{xz}$ for all samples are listed in Table SII. Note that the out-of-plane driving fields are complex due to the phase difference of $\epsilon_{xz,0}$ with respect to $\epsilon_{xx,0}$. By reversing the direction of the SAW $k_{\mathrm{S21}} \to k_{\mathrm{S12}}$ (or $k \to -k$) the elliptical motion of the lattice displacement in the xz-plane, the phase difference between $\epsilon_{xz,0}$ and $\epsilon_{xx,0}$ and the helicity of the driving fields change [8], expressed by the sign of $\tilde{a}_{xz}$ ($\tilde{a}_{xz} > 0$ for $k_{\mathrm{S21}}$, $\tilde{a}_{xz} < 0$ for $k_{\mathrm{S12}}$). In combination with the fixed rotational sense of the magnetization precession, the SAW-SW helicity mismatch effect arises.

Following Ref. [9, 10], $|u_{z,0}|$ is a function of the SAW power $P_{\mathrm{SAW}}$

$$|u_{z,0}(x)| = \sqrt{\frac{1}{R\,\omega W}}\sqrt{P_{\mathrm{SAW}}(x)}, \tag{3}$$

with the aperture of the IDT $W$ and the numerically calculated constant $R = 1.40 \times 10^{11}$ J/m$^3$ for a Y-cut Z-propagation $LiNbO_3$ substrate [9]. With Eqs. (2) and (3), Eq. (1) can be expressed as a function of $P_{\mathrm{SAW}}$

$$\mathbf{h}(x,t) = \begin{pmatrix}\tilde{h}_1\\ \tilde{h}_2\end{pmatrix}\sqrt{\frac{k^2}{R\,\omega W}}\sqrt{P_{\mathrm{SAW}}(x)}\ \mathrm{e}^{i(kx-\omega t)}, \tag{4}$$

with

$$\begin{pmatrix} \tilde{h}_1 \\ \tilde{h}_2 \end{pmatrix} = \begin{pmatrix} 2\frac{b_{xz}}{\mu_0}\cos\phi_0 \\ 2\frac{b_{xx}}{\mu_0}\cos\phi_0\sin\phi_0 \end{pmatrix}, \tag{5}$$

where we have substituted $b_{xx} = b_1\tilde{a}_{xx}$ and $b_{xz} = b_2\tilde{a}_{xz}$.

**Fit equation**

Following Ref. [2], the power that is used to drive magnetization precession is

$$P_{\mathrm{abs}} = \frac{1}{2}\omega\mu_0 \int_{V_0} \mathrm{Im}\left\{\mathbf{h}^*\bar{\chi}\mathbf{h}\right\} \mathrm{d}V_0 \approx \frac{1}{2}\omega\mu_0(Wd)\int_0^{l_\mathrm{f}} \mathrm{Im}\left\{\mathbf{h}^*\bar{\chi}\mathbf{h}\right\} \mathrm{d}x \tag{6}$$

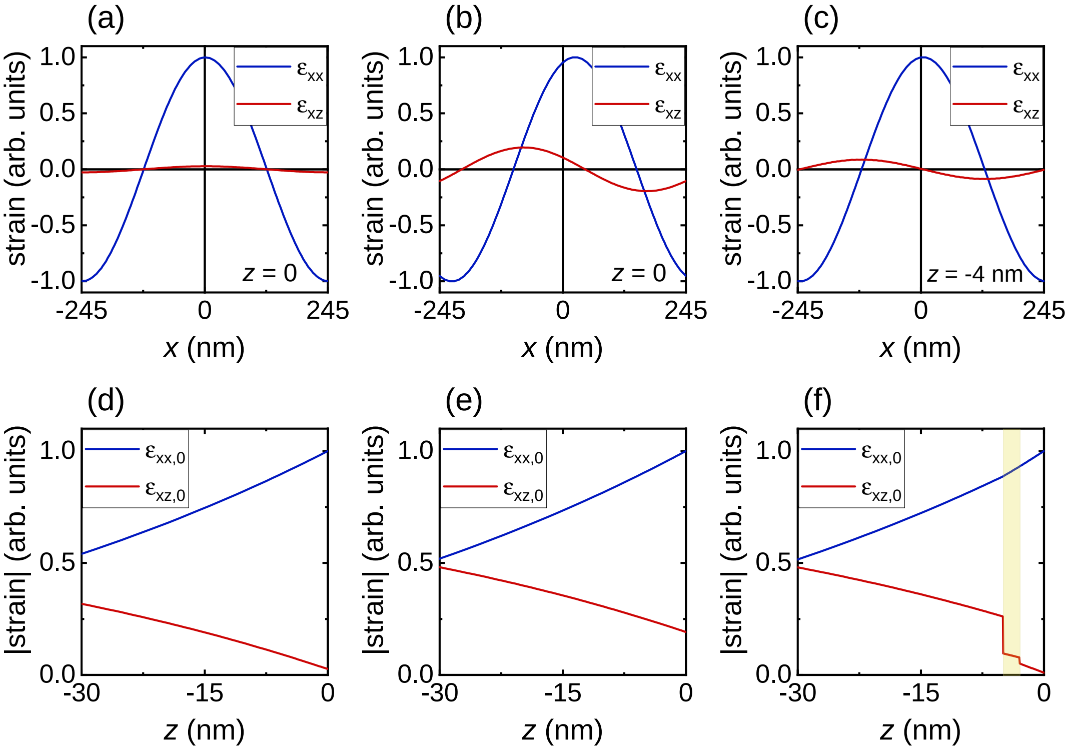


FIG. S2. Finite element simulation, carried out with Comsol [4] at ∼6.9 GHz to calculate the strain components of a Rayleigh wave for a pure $LiNbO_3$ substrate (a, d), a pure $LiNbO_3$ substrate with a perfectly conducting overlayer of zero thickness (b, e) and a $LiNbO_3$/CoFeB(2)/$Si_3N_4$(3) sample (c, f). The strain in the x-direction $\epsilon_{xx}(x), \epsilon_{xz}(x)$ is shown in panels (a-c) for one wavelength at an arbitrary point in time. The absolute value of the strain in the z-direction is depicted in panel (d-f). The top surface of the samples is located at $z = 0$ and the yellow area in panel (f) indicates the position of the magnetic thin film.

TABLE SII. Results of the finite element method simulation. The normalized complex amplitudes of the longitudinal and vertical shear strain components are given by $\tilde{a}_{xx}$ and $\tilde{a}_{xz}$. The final row determines the magnitude of the magnetorotational coupling, discussed in Fig. S6(b). The errors for $\tilde{a}_{xx}$, $\tilde{a}_{xz}$ and $\frac{\omega_{xz,0}}{|u_{z,0}||k|}$ are assumed to be in the order of ±20%, ±50% and ±20%, resulting mainly from the assumed thin film properties in Table SI.

| | CoFeB(1.4)/Pt | CoFeB(1.7)/Pt | CoFeB(2)/Pt | CoFeB(3.5)/Pt | CoFeB(5)/Pt | CoFeB(2) |
|---|---|---|---|---|---|---|
| $\tilde{a}_{xx} = \frac{\epsilon_{xx,0}}{|u_{z,0}||k|}$ | 0.46 | 0.46 | 0.46 | 0.46 | 0.45 | 0.49 |
| $\tilde{a}_{xz} = \frac{\epsilon_{xz,0}}{|u_{z,0}||k|}$ | $\pm i0.037$ | $\pm i0.038$ | $\pm i0.039$ | $\pm i0.043$ | $\pm i0.048$ | $\pm i0.042$ |
| $\frac{\omega_{xz,0}}{|u_{z,0}||k|}$ | $\mp i0.97$ | $\mp i0.96$ | $\mp i0.96$ | $\mp i0.96$ | $\mp i0.96$ | $\mp i0.96$ |

with the volume $V_0$, thickness $d$, length $l_\mathrm{f}$ of the magnetic film and the magnetic susceptibility $\bar{\chi}$. We assumed constant magnetic driving fields across the magnetic film thickness, which is a good approximation for the characterized ultrathin magnetic films, as shown in Fig. S2.

With increasing propagation of the SAW through the magnetic film, the power of the SAW $P_\mathrm{SAW} = P_0 - P_\mathrm{abs}$ decreases with respect to the initial power $P_0$. Combining Eqs. (4) and (6), we obtain the differential equation

$$P_\mathrm{abs} = \frac{1}{2}\omega\mu_0(Wd)\left(\frac{k^2}{R\omega W}\right)\mathrm{Im}\left\{\begin{pmatrix}\tilde{h}_1\\ \tilde{h}_2\end{pmatrix}^{*}\bar{\chi}\begin{pmatrix}\tilde{h}_1\\ \tilde{h}_2\end{pmatrix}\right\}\int_0^{l_\mathrm{f}}(P_0 - P_\mathrm{abs})\,\mathrm{d}x, \tag{7}$$

with the solution

$$P_\mathrm{abs} = P_0\left\{1-\exp\left\{-C\,\mathrm{Im}\left[\begin{pmatrix}\tilde{h}_1\\ \tilde{h}_2\end{pmatrix}^{*}\bar{\chi}\begin{pmatrix}\tilde{h}_1\\ \tilde{h}_2\end{pmatrix}\right]\right\}\right\}$$
$$\text{and } C = \frac{1}{2}\mu_0 V_0\left(\frac{k^2}{RW}\right). \tag{8}$$

Following the "Landau–Lifshitz–Gilbert approach" of Ref. [2], the magnetic susceptibility tensor is calculated by solving the Landau–Lifshitz–Gilbert equation for small deviations of the magnetization from its equilibrium orientation in a rotated 123-coordinate system. We assume that the effective magnetic field $\mu_0\mathbf{H}_\mathrm{eff}$ is caused by the magnetoacoustic driving fields, external magnetic field, in-plane uniaxial magnetic anisotropy, magnetic shape anisotropy, effective dipolar field [11], magnetic exchange interaction, and DMI effective field [12]. For the effective field in the right-handed 123-coordinate system, with the 3-axis

(1-axis) being parallel to the magnetization (film normal) direction, we obtain

$$\mu_0\mathbf{H}_{\mathrm{eff},123} = \mu_0 \begin{pmatrix} h_{\mathrm{oop}} \\ h_{\mathrm{ip}} \\ 0 \end{pmatrix} + \mu_0\mathbf{H}_{123} + \mu_0 H_{\mathrm{ani}}(\mathbf{m}_{123}\cdot\mathbf{u}_{123})\mathbf{u}_{123} + \mu_0 H_{\mathrm{k}} \begin{pmatrix} m_1 \\ 0 \\ 0 \end{pmatrix}$$
$$- \mu_0 M_{\mathrm{s}} \begin{pmatrix} G_0 m_1 \\ (1-G_0) m_2 \sin^2(\phi_0) \\ 0 \end{pmatrix} - \frac{2A}{M_{\mathrm{s}}} k^2 \begin{pmatrix} m_1 \\ m_2 \\ 0 \end{pmatrix} + i\frac{2D_{\mathrm{eff}}}{M_{\mathrm{s}}} k \sin\phi_0 \begin{pmatrix} -m_2 \\ m_1 \\ 0 \end{pmatrix}, \quad (9)$$

where $\mathbf{H}_{123}, \mathbf{m}_{123}$, and $\mathbf{u}_{123}$ are external magnetic field vector, unity magnetization vector and unity in-plane easy axis field vector in the 123-coordinate system, respectively. Furthermore, $H_{\mathrm{ani}}$ is the in-plane easy axis field magnitude, $H_{\mathrm{k}}$ is the magnitude of the out-of-plane surface anisotropy field, that partly counteracts the magnetic shape anisotropy, $M_{\mathrm{s}}$ describes the saturation magnetization, $G_0 = \left(1 - \mathrm{e}^{-|k|d}\right) / (|k|d)$ is a dipolar spin wave term [11], $A$ is the magnetic exchange stiffness and $D_{\mathrm{eff}}$ is the effective DMI constant. The solution of the linearized Landau–Lifshitz–Gilbert equation $\frac{\partial \mathbf{m}_{123}}{\partial t} = \gamma\mu_0\mathbf{H}_{\mathrm{eff},123} \times \mathbf{m}_{123} + \alpha\mathbf{m}_{123} \times \frac{\partial \mathbf{m}_{123}}{\partial t}$ is concisely formulated with the inverse magnetic susceptibility

$$\begin{aligned}
\bar{\chi}^{-1} &= \frac{1}{M_{\mathrm{s}}} \begin{pmatrix} \chi^I_{11} & \chi^I_{12} \\ \chi^I_{21} & \chi^I_{22} \end{pmatrix} \\
\chi^I_{11} &= H\cos(\phi_0 - \phi_{\mathrm{H}}) + \frac{2A}{\mu_0 M_{\mathrm{s}}} k^2 + M_{\mathrm{s}} G_0 - H_{\mathrm{k}} + H_{\mathrm{ani}} \cos^2(\phi_0 - \phi_{\mathrm{ani}}) - i\frac{\alpha\omega}{\mu_0\gamma} \\
\chi^I_{12} &= -\chi^I_{21} = i\left(\frac{\omega}{\mu_0\gamma} + \frac{2D_{\mathrm{eff}}}{\mu_0 M_{\mathrm{s}}} k \sin(\phi_0)\right) \\
\chi^I_{22} &= H\cos(\phi_0 - \phi_{\mathrm{H}}) + \frac{2A}{\mu_0 M_{\mathrm{s}}} k^2 + M_{\mathrm{s}}(1 - G_0)\sin^2(\phi_0) + H_{\mathrm{ani}} \cos(2(\phi_0 - \phi_{\mathrm{ani}})) - i\frac{\alpha\omega}{\mu_0\gamma},
\end{aligned} \quad (10)$$

where $\phi_{\mathrm{H}}$ and $\phi_{\mathrm{ani}}$ are the directions of the external magnetic field $H$ and of the in-plane anisotropy easy-axis, with respect to the x-axis. Additionally, $\alpha$ is the spin wave damping constant. Finally, $\gamma$ is the gyromagnetic ratio. We invert matrix $\bar{\chi}^{-1}$ in Eq. (10) to obtain

$\bar{\chi}$ which we insert in Eq. (8) to find for real $\tilde{h}_2$ and imaginary $\tilde{h}_1$

$$P_{\text{abs}} = P_0 \Bigg\{ 1 - \exp\Bigg\{ -CM_{\text{s}} \frac{\alpha H_\omega}{\left[(H_\omega + H_{\text{DMI}})^2 - H_{11}H_{22} + (\alpha H_\omega)^2\right]^2 + \left[\alpha H_\omega (H_{11} + H_{22})\right]^2}$$
$$\times \Big\{ \left[(H_\omega + H_{\text{DMI}})^2 + H_{11}^2 + (\alpha H_\omega)^2\right] \left[\text{Re}(\tilde{h}_2)\right]^2$$
$$+ \left[(H_\omega + H_{\text{DMI}})(H_{11} + H_{22})\right] \left[-2\,\text{Re}(\tilde{h}_2)\,\text{Im}(\tilde{h}_1)\right]$$
$$+ \left[(H_\omega + H_{\text{DMI}})^2 + H_{22}^2 + (\alpha H_\omega)^2\right] \left[\text{Im}(\tilde{h}_1)\right]^2 \Big\} \Bigg\} \Bigg\} \tag{11}$$

with the substitutions

$$H_\omega = \frac{\omega}{\mu_0 \gamma}, \quad H_{\text{DMI}} = \frac{2D_{\text{eff}}}{\mu_0 M_{\text{s}}} k \sin(\phi_0),$$
$$H_{11} = \text{Re}\left(\chi_{11}^I\right), \quad H_{22} = \text{Re}\left(\chi_{22}^I\right). \tag{12}$$

Eq. (2) in the main text, which is the spin wave dispersion relation, is obtained by setting $\det\left(\bar{\chi}^{-1}\right) = 0$ and taking the real part of the solution for small $\alpha$ and $\phi_0 = \phi_{\text{H}}$

$$\omega = \gamma \mu_0 \left( \sqrt{H_{11}H_{22}} - H_{\text{DMI}} \right). \tag{13}$$

Finally, the experimentally determined relative change of the SAW transmission $\Delta S_{ij}$ on the logarithmic scale is fitted with Eq. (11) and

$$\Delta S_{ij} = 10\,\text{lg}\left(\frac{P(\mu_0 H)}{1\text{ mW}}\right) - 10\,\text{lg}\left(\frac{P(-200\text{ mT})}{1\text{ mW}}\right) = 10\,\text{lg}\left(\frac{P_0 - P_{\text{abs}}}{P_0}\right), \tag{14}$$

where we assume for our experiments $P(-200\text{ mT}) = P_0$ (no SAW-SW interaction far off SW resonance). In this way, the initial SAW power $P_0$ cancels and we fit directly the exponent of Eq. (11), that contains the information about the driving fields and the magnetic susceptibility.

## [S.3] FITTING PROCEDURE

The SAW transmission $\Delta S_{ij}(\mu_0 H, \phi_{\text{H}})$ is globally fitted with Eqs. (11,14), following the routine:

- The minima $\mu_0 H_{\text{res}}(\phi_{\text{H}})$ of $\Delta S_{ij}(\mu_0 H, \phi_{\text{H}})$ for $\mu_0 H > 0$ are extracted and fitted with the spin wave dispersion relation Eq. (13). The used values for $\gamma$ were determined

by broadband FMR. Because the spin wave dispersion relation is deduced by the assumption $\phi_0 = \phi_{\mathrm{H}}$, this fit is only a good approximation for $\mu_0 H_{\mathrm{res}} \gg \mu_0 H_{\mathrm{ani}}$, as shown exemplarily in Fig. S3(a) for the CoFeB(2)/Pt film.

- The fit values of the previous step $(D_{\mathrm{eff}}, H_{\mathrm{k}}, \phi_{\mathrm{ani}}, H_{\mathrm{ani}})$ are the start parameters for the global fit with Eqs. (11,14). The global fit additionally considers the field drag effect $\phi_0 \neq \phi_{\mathrm{H}}$. This effect arises due to an uniaxial in-plane anisotropy present in the sample which is attributed to anisotropic thermal expansion of $LiNbO_3$ during deposition. Consideration of this uniaxial anisotropy is important for the simulation shown in Fig. 4 in the main text. The global fit is carried out iteratively for anisotropy parameter tuples $(\phi_{\mathrm{ani}}, H_{\mathrm{ani}})$, with a minimum increment of (0.1°, 0.1 mT):

  1. For one tuple $(\phi_{\mathrm{ani}}, H_{\mathrm{ani}})$ the orientation of the in-plane equilibrium magnetization $\phi_0(\mu_0 H, \phi_{\mathrm{H}})$ is calculated by energy minimization of Zeeman-energy and uniaxial in-plane anisotropy energy $G = -\mu_0 H \cos(\phi_{\mathrm{H}} - \phi_0) - \frac{1}{2}\mu_0 H_{\mathrm{ani}} \cos^2(\phi_{\mathrm{ani}} - \phi_0)$ [2].
  2. The global fit with the fit parameters $(D_{\mathrm{eff}}, H_{\mathrm{k}}, \alpha, b_{xx}, b_{xz})$ is carried out. Because $H_{\mathrm{k}}$ and the magnetic exchange stiffness $A$ are strongly correlated, a simultaneous fit of both parameters is not possible and we use $A = 11$ pJ/m from literature [13].
  3. The deviation of fit and experiment is further minimized by varying $(\phi_{\mathrm{ani}}, H_{\mathrm{ani}})$, according to a bisection search method and repeating the previous steps 1-3.

The quality of the final fit result in terms of resonance fields $\mu_0 H_{\mathrm{res}}(\phi_{\mathrm{H}})$ and deviation of fit and experiment $\Delta S_{21}^{\mathrm{fit}} - \Delta S_{21}^{\mathrm{exp}}$ for the CoFeB(2)/Pt film is depicted in Figs. S3(a,b).

## [S.4] ADDITIONAL FIT RESULTS

We find overall excellent agreement between experiment and fit with reasonable fit parameters summarized in Table SIII. The determined **saturation magnetization** values for CoFeB(2) and CoFeB(1.4–2.0)/Pt are in good agreement with literature [14]. We attribute the higher $M_{\mathrm{s}}$ of the CoFeB(2)/Pt samples in comparison to the CoFeB(2) sample to proximity polarization of the Pt layer [15, 16]. The thicker samples were fabricated in a second sputter run and show higher values for $M_{\mathrm{s}}$. Presumably the composition of the magnetic thin films has slightly changed.

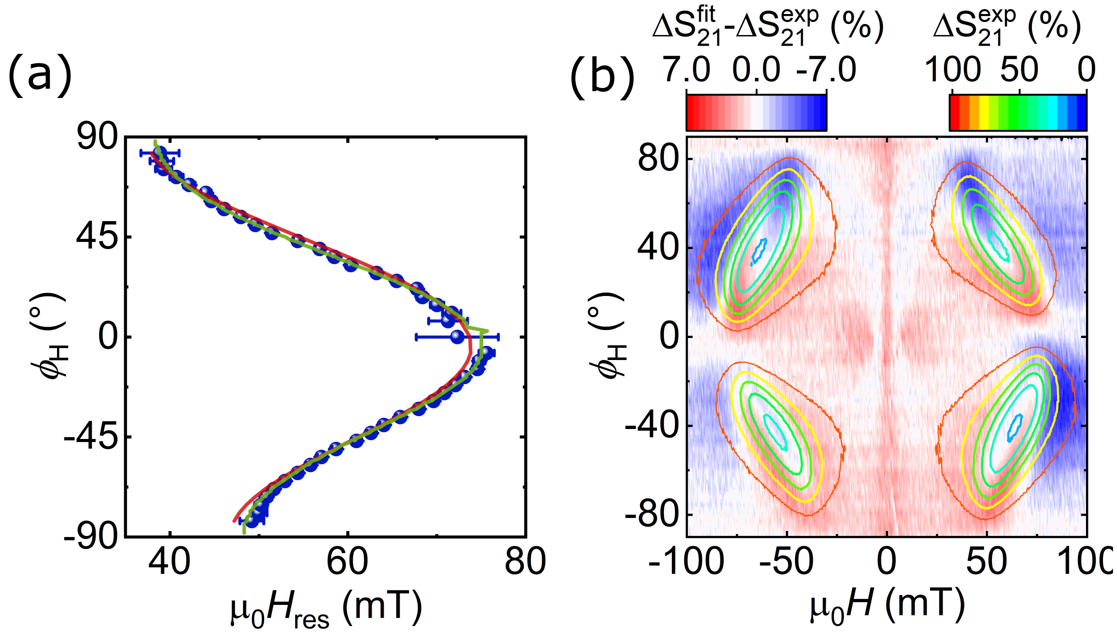


FIG. S3. Demonstration of the quality of the fitting procedure for the CoFeB(2 nm)/Pt film at 6.88 GHz. (a) Whereas the resonance fields of the spin wave dispersion fit (red curve) deviate slightly from the experimental data $\Delta S_{21}$ (blue dots), the full model (green curve), which additionally considers the field drag effect, shows excellent agreement with the experiment. (b) Deviation of fit and experiment, linearly scaled, is at maximum 6.6%, while the experimentally determined SAW transmission drops from 100% to 12.5% at resonance.

Interestingly, all CoFeB films show an unusual high **in-plane magnetic anisotropy** with an easy axis aligned parallel to the y-axis of the coordinate system. Because this anisotropy is also present in the CoFeB(2) film and it decreases with the magnetic film thickness, we attribute this anisotropy to the $LiNbO_3$/CoFeB interface, being induced by the anisotropic $LiNbO_3$ single-crystal.

The **chirality** which is favored by the DMI in our samples is discussed in the following section. Note that the definition of the sign of $D_{\text{eff}}$ is based on Ref. [12]. Figure S4 illustrates a cross-sectional view of the xz-plane of Fig. S1 for $\phi_0 = \phi_H = +90°$, $H > 0$ and $k_{S21}$. In the experiment, the direction of $k_{S21}$ is given by the ports of the vector network analyzer and the magnetic field direction was determined by the procedure, described in Ref. [17]. According to Fig. 2(b) in the main text, the DMI lowers the resonant field for $\phi_H, H > 0$, $k_{S21}$ and $f = 6.88$ GHz, which corresponds to a DMI induced increase of the resonance frequency in

TABLE SIII. Summary of the film parameters and fitting results. $l_f$ is the length of the magnetic films and $M_s$ is determined by SQUID-VSM magnetometry. The other values are obtained by fitting the SAW transmission data $\Delta S_{21}$ with Eqs. (11, 14) at the frequency $f$ of the SAW. The errors are the standard errors of the global fit. For $\phi_{ani}$ and $\mu_0 H_{ani}$ the errors are assumed to be below 0.2° and 0.2 mT.

| | CoFeB(1.4)/Pt | CoFeB(1.7)/Pt | CoFeB(2)/Pt | CoFeB(3.5)/Pt | CoFeB(5)/Pt | CoFeB(2) |
|---|---|---|---|---|---|---|
| $l_f$ ($\mu$m) | 1250 | 1250 | 1250 | 750 | 750 | 1250 |
| $f$ (GHz) | 6.87 | 6.87 | 6.88 | 6.88 | 6.77 | 6.9 |
| $M_s$ (kA/m) | 1320 | 1306 | 1262 | 1534 | 1504 | 1125 |
| $\phi_{ani}$ (°) | 88.8 | 90.5 | 87.7 | 83.9 | 83.2 | 88.9 |
| $\mu_0 H_{ani}$ (mT) | 8.4 | 7.2 | 7.1 | 4.2 | 4.8 | 6.0 |
| $H_k$ (kA/m) | $837.9 \pm 0.07$ | $772.4 \pm 0.05$ | $659.5 \pm 0.05$ | $629.3 \pm 0.1$ | $483.8 \pm 0.2$ | $505 \pm 0.01$ |
| $D_{eff}$ ($\mu$J/m$^2$) | $-592 \pm 1.1$ | $-484 \pm 0.7$ | $-424 \pm 0.7$ | $-357 \pm 1.3$ | $-285 \pm 2.3$ | $-32 \pm 0.1$ |
| $\alpha$ ($10^{-3}$) | $55.3 \pm 0.05$ | $45.8 \pm 0.03$ | $37.6 \pm 0.03$ | $20.7 \pm 0.04$ | $17.8 \pm 0.05$ | $10.7 \pm 0.01$ |
| $-b_{xx}$ (T) | $3.119 \pm 0.001$ | $2.948 \pm 0.001$ | $3.021 \pm 0.001$ | $2.936 \pm 0.002$ | $3.025 \pm 0.003$ | $1.963 \pm 0.001$ |
| $-b_{xz}$ (T) | $i0.560$ | $i0.581$ | $i0.692$ | $i0.983$ | $i1.079$ | $i0.589$ |
| Error($b_{xz}$) (T) | $\pm i0.001$ | $\pm i0.0019$ | $\pm i0.0019$ | $\pm i0.004$ | $\pm i0.007$ | $\pm i0.001$ |

a fixed external magnetic field. The alignment of wave vector and magnetization determine the spatial chirality of the SW [18], which is counter-clockwise in the x-direction for $k_{S21}$ in Fig. S4. According to Ref. [18], a DMI induced increase of the SW frequency indicates that the spatial chirality of the SW is not favored by the DMI. Thus, the DMI favors clockwise chirality in our samples. This corresponds to a right-handed chirality in the x-direction, with respect to magnetization direction and as depicted e.g. in Ref. [19].

According to Eq. (13), the interfacial DMI causes a pronounced shift of the resonant magnetic fields $H_{res}$ for counterpropagating magnetoacoustic waves. As shown in Fig. S5(a) and in contrast to Fig. 3(a) in the main text, the resonant fields of $\Delta S_{21}$ and $\Delta S_{12}$ of the CoFeB(2) sample are not shifted with respect to each other.

The **effective magnetization** $M_{eff} = M_s - H_k$ is one important parameter, which can be determined by SAW assisted SW spectroscopy. The $M_{eff}$ values obtained from the global fit show excellent agreement with those obtained by broadband FMR. The $M_{eff}$ obtained

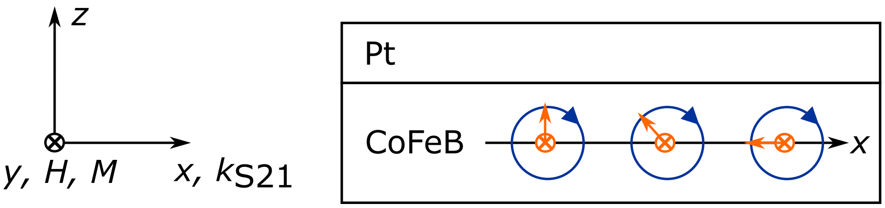


FIG. S4. Cross-sectional view of the xz-plane of Fig. S1 for $\phi_0 = \phi_H = +90°$, $H > 0$. The SW with the wave vector $k_{S21}$ is propagating in the x-direction. The right-handed sense of the magnetization precession (blue) dictates the SW modal profile (orange: dynamic magnetization components), showing counter-clockwise chirality in the x-direction, as depicted for an arbitrary point in time.

by both techniques are plotted for the CoFeB($d$)/Pt series as a function of the inverse film thickness in Fig. S5(b). $M_{\text{eff}}$ scales linearly with $1/d$, revealing the interface character of the surface anisotropy energy. The intercept with the x-axis corresponds to the reorientation phase transition at $d = (1.1 \pm 0.2)$ nm. The saturation magnetization $M_s$ is higher than the intercept with the y-axis at $(1190 \pm 70)$ kA/m. We attribute this to a magnetic volume anisotropy in our samples.

In Fig. S6(a) we show the Gilbert **damping** $\alpha^{\text{FMR}}$ determined by out-of-plane broadband magnetic resonance on the CoFeB/Pt bilayers as a function of $1/d$. To compare these damping constants to those obtained from our fits to the magnetoacoustic surface wave (MASW) spectroscopy data, we must consider the effect of inhomogeneous broadening $\mu_0 \Delta H$. To this end, we define the damping constant $\alpha_{\text{eff}}^{\text{FMR}} = \frac{\gamma}{2\omega}\mu_0 \Delta H + \alpha^{\text{FMR}}$ with $\omega$ being the SAW angular frequency. This can now be compared to the effective SW damping constant $\alpha_{\text{eff}}^{\text{SAW}} \equiv \alpha$, obtained from our MASW data. We find generally good agreement between $\alpha_{\text{eff}}^{\text{SAW}}$ and $\alpha_{\text{eff}}^{\text{FMR}}$. Both parameters show the same linear dependence on $1/d$, in accordance with a spin-pumping mechanism [20]. The values of $\alpha_{\text{eff}}^{\text{SAW}}$ are systematically higher than $\alpha_{\text{eff}}^{\text{FMR}}$. This is attributed to two-magnon scattering, which is present in the in-plane magnetoacoustic measurements, but is suppressed in out-of-plane broadband FMR [21]. The generally good agreement of $\alpha_{\text{eff}}^{\text{SAW}}$ and $\alpha_{\text{eff}}^{\text{FMR}}$ is in contrast to previous findings [2, 22], which might be due to the higher SAW frequencies employed here.

As shown in Fig. 3(c) of the main text, the **driving field fit parameter** $|b_{xz}|$ increases with film thickness for the CoFeB($d$)/Pt series. The origin of this behavior is discussed

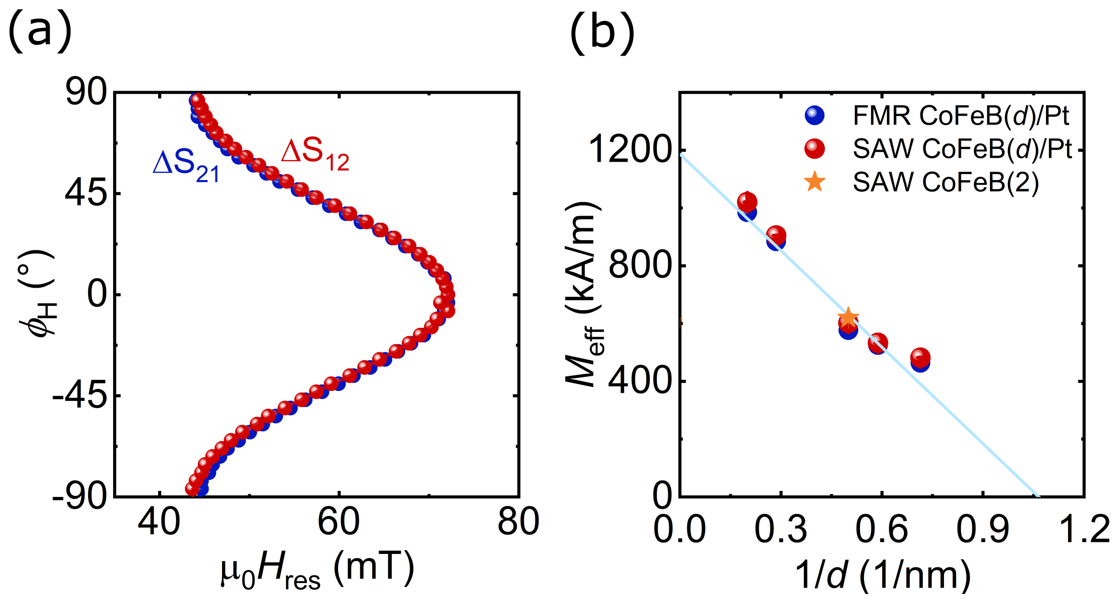


FIG. S5. (a) Angular dependence of the resonance fields of the CoFeB(2) sample. (b) The effective magnetization $M_{\mathrm{eff}}$ as a function of the inverse of the magnetic film thickness. $M_{\mathrm{eff}}$ was determined with SAW assisted SW spectroscopy and broadband FMR. Both show excellent agreement. The blue line is the linear fit to the FMR data.

in more detail in Fig. S6(b). First, we calculate the expected magnetoelastic magnitude $b_{xz,\mathrm{ME}} = b_2 \tilde{a}_{xz}$. With the fit value $b_{xx} = b_1 \tilde{a}_{xx}$ of Table SIII and the value of $\tilde{a}_{xx}$ from the finite element method (FEM) simulation in Table SII, we get the magnetoelastic constant $b_1$. Assuming a polycrystalline/amorphous CoFeB film ($b_2 = b_1$) and taking $\tilde{a}_{xz}$ from the FEM simulation, we calculate the expected magnetoelastic contribution $b_{xz,\mathrm{ME}}$. The purely magnetoelastic contributions are too small to explain the fit value $b_{xz}$.

In a recent related study, the high value of $b_{xz}$ is explained by another mechanism, the so-called magnetorotational coupling, which induces a driving field with the same symmetry as the shear magnetoelastic driving field [23]. The additional contribution due to magnetorotational coupling is given by $b_{xz,\mathrm{MR}} = -B_{\mathrm{u}} \frac{\omega_{xz,0}}{|u_{z,0}||k|}$. Here, the uniaxial effective out-of-plane anisotropy $B_{\mathrm{u}} = -\frac{1}{2}\mu_0 M_{\mathrm{eff}}$ and the complex amplitude $\omega_{xz,0}$ of the rotation tensor element $\omega_{xz} = \frac{1}{2}\left(\frac{\partial u_x}{\partial z} - \frac{\partial u_z}{\partial x}\right)$ determine the magnitude of $b_{xz,\mathrm{MR}}$. The expected $b_{xz,\mathrm{MR}}$ in Fig. S6(b) is obtained by extracting $\frac{\omega_{xz,0}}{|u_{z,0}||k|}$ from the FEM simulation (Table SII) and calculating $B_{\mathrm{u}}$ with the corresponding values in Table SIII. We find that both mechanisms reproduce the trend of increasing $b_{xz}$ with increasing $d$, but underestimate $b_{xz}$ by a factor $2-3$. How-

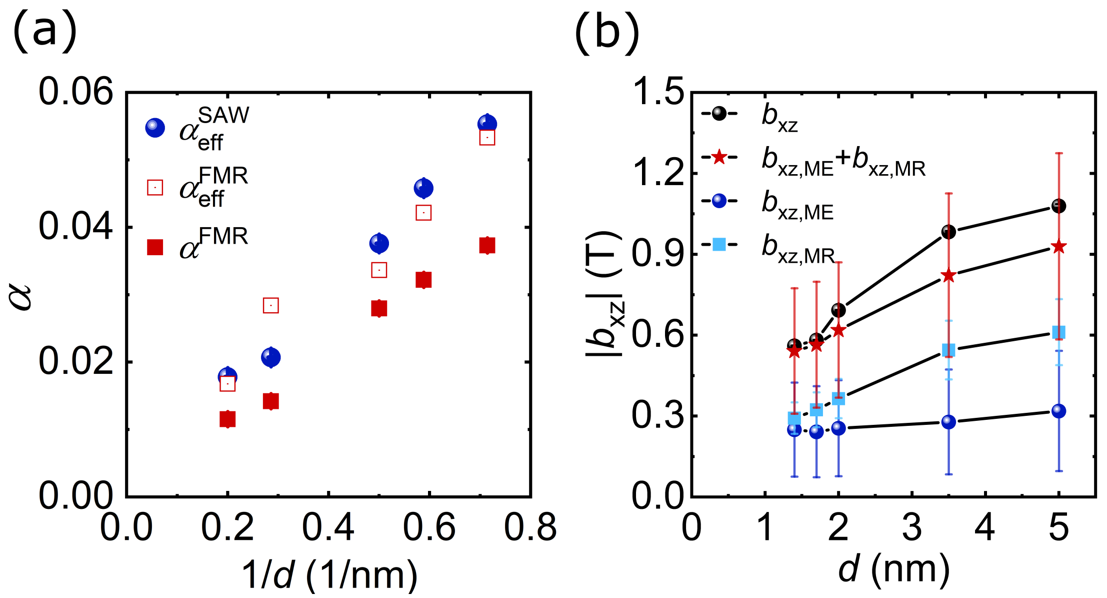


FIG. S6. (a) The SW damping constant as a function of the inverse of the magnetic film thickness. The error bars are smaller than the symbol sizes. (b) The fit parameter $b_{xz}$, ruling the magnitude of the out-of-plane driving field, is compared with the theoretical expectations for the CoFeB($d$)/Pt thickness series. The purely magnetoelastic contribution $b_{xz,\mathrm{ME}}$ with the magnetoelastic constant $b_2 = b_1$, taken from the experiment, is too small to explain the experimental results. Additionally, the expected magnitude $b_{xz,\mathrm{MR}}$, caused by magnetorotational coupling and the sum of both mechanisms is depicted.

ever, both mechanisms are expected to be in phase, that is why we have to compare the constructive interference $b_{xz,\mathrm{ME}} + b_{xz,\mathrm{MR}}$ with the experimental data. Within the large error bars $b_{xz,\mathrm{ME}} + b_{xz,\mathrm{MR}}$ agrees with the experimental data. We conclude that both effects are present and contribute to the observed $b_{xz}$.

---

* matthias.kuess@physik.uni-augsburg.de.

† Present address: Fachbereich Physik, Technische Universität Kaiserslautern, 67663 Kaiserslautern, Germany

[1] D. P. Morgan, *Surface Acoustic Wave Filters: With Applications to Electronic Communications and Signal Processing*, 2nd ed. (Elsevier, Amsterdam, 2007).

[2] L. Dreher, M. Weiler, M. Pernpeintner, H. Huebl, R. Gross, M. S. Brandt, and S. T. B.

Goennenwein, Phys. Rev. B **86**, 134415 (2012).

[3] E. D. S. Nysten, Y. H. Huo, H. Yu, G. F. Song, A. Rastelli, and H. J. Krenner, J. Phys. D **50**, 43LT01 (2017).

[4] COMSOL Multiphysics® v. 5.4. `www.comsol.com`. COMSOL AB, Stockholm, Sweden.

[5] We assume a Poisson ratio in the order of cobalt and iron. For the Youngs‘s modulus we take the value from Ref. [6] for $Co_{62}Fe_{23}B_{15}$. The density is assumed to be the weighted average of the density of the elements.

[6] J. M. Barandiarán, J. Gutiérrez, Z. Kaczkowski, and D. de Cos, J. Non-Cryst. Solids **329**, 43 (2003).

[7] S. Datta, *Surface Acoustic Wave Devices* (Prentice-Hall, Englewood Cliffs NJ, 1986).

[8] R. Sasaki, Y. Nii, Y. Iguchi, and Y. Onose, Phys. Rev. B **95**, 020407 (2017).

[9] W. P. Robbins, IEEE Trans. Son. Ultrason. **24**, 339 (1977).

[10] D. Labanowski, A. Jung, and S. Salahuddin, Appl. Phys. Lett. **108**, 022905 (2016).

[11] B. A. Kalinikos and A. N. Slavin, J. Phys. C **19**, 7013 (1986).

[12] J.-H. Moon, S.-M. Seo, K.-J. Lee, K.-W. Kim, J. Ryu, H.-W. Lee, R. D. McMichael, and M. D. Stiles, Phys. Rev. B **88**, 184404 (2013).

[13] J. Cho, J. Jung, K.-E. Kim, S.-I. Kim, S.-Y. Park, M.-H. Jung, and You Chun-Yeol, J. Magn. Magn. Mater. **339**, 36 (2013).

[14] J. Cho, N.-H. Kim, S. Lee, J.-S. Kim, R. Lavrijsen, A. Solignac, Y. Yin, D.-S. Han, N. J. J. van Hoof, H. J. M. Swagten, B. Koopmans, and C.-Y. You, Nat. Commun. **6**, 7635 (2015).

[15] M. Suzuki, H. Muraoka, Y. Inaba, H. Miyagawa, N. Kawamura, T. Shimatsu, H. Maruyama, N. Ishimatsu, Y. Isohama, and Y. Sonobe, Phys. Rev. B **72**, 054430 (2005).

[16] H.-Y. Lee, S. Kim, J.-Y. Park, Y.-W. Oh, S.-Y. Park, W. Ham, Y. Kotani, T. Nakamura, M. Suzuki, T. Ono, K.-J. Lee, and B.-G. Park, APL Mater. **7**, 031110 (2019).

[17] M. Schreier, G. E. W. Bauer, V. I. Vasyuchka, J. Flipse, K. Uchida, J. Lotze, V. Lauer, A. V. Chumak, A. A. Serga, S. Daimon, T. Kikkawa, E. Saitoh, B. J. van Wees, B. Hillebrands, R. Gross, and S. T. B. Goennenwein, J. Phys. D **48**, 025001 (2014).

[18] H. T. Nembach, J. M. Shaw, M. Weiler, E. Jué, and T. J. Silva, Nat. Phys. **11**, 825 (2015).

[19] G. Chen, J. Zhu, A. Quesada, J. Li, A. T. N'Diaye, Y. Huo, T. P. Ma, Y. Chen, H. Y. Kwon, C. Won, Z. Q. Qiu, A. K. Schmid, and Y. Z. Wu, Phys. Rev. Lett. **110**, 177204 (2013).

[20] Y. Tserkovnyak, A. Brataas, and G. E. W. Bauer, Phys. Rev. Lett. **88**, 117601 (2002).

[21] X. Liu, W. Zhang, M. J. Carter, and G. Xiao, J. Appl. Phys. **110**, 033910 (2011).

[22] P. G. Gowtham, T. Moriyama, D. C. Ralph, and R. A. Buhrman, J. Appl. Phys. **118**, 233910 (2015).

[23] M. Xu, K. Yamamoto, J. Puebla, K. Baumgaertl, B. Rana, K. Miura, H. Takahashi, D. Grundler, S. Maekawa, and Y. Otani, Sci. Adv. **6**, eabb1724 (2020).
